# Supplementary material for: Chain of Attack: On the Robustness of Vision-Language Models Against Transfer-Based Adversarial Attacks
Source: arXiv:2411.15720 source file (2024-11-24)
Supplement: Supplementary file 1 [file supp.tex]

\clearpage
\setcounter{page}{1}
\maketitlesupplementary

\begin{table*}[t]  

 %控制行高  
\setlength{\tabcolsep}{0.7mm}
\centering  
%\fontsize{9}{10}\selectfont  % \fontsize{字体尺寸}{行间距}\selectfont 
\begin{threeparttable}  
		  
%\begin{tabular}{cc|cccccc|ccc}  
%p{3cm} 
%>{\centering\arraybackslash}p{1.2cm} % 列居中+设定列宽为1.2cm
\begin{tabular}{c|>{\centering\arraybackslash}p{1.4cm}>{\centering\arraybackslash}p{1.4cm}>{\centering\arraybackslash}p{1.4cm}>{\centering\arraybackslash}p{1.4cm}>{\centering\arraybackslash}p{1.4cm}>{\centering\arraybackslash}p{1.4cm}}  
    \toprule\hline
    \multirow{2}{*}{\bf \textsc{Attacking method}}&
    \multicolumn{6}{c}{\bf \textsc{CLIP Score / Text Encoder}}\cr

    %\cline{3-8}\cline{9-11}
    \cmidrule(lr){2-7}
    & RN-50 & RN-101 & ViT-B/16 & ViT-B/32 & ViT-L/14 & Ensemble\\
    \hline
    Clean image
    & 41.7&	41.5&	42.9&	44.6&	30.5&	40.2\\
    Ours CoA/PGD-10 
    &63.1	&61.5	&64.5	&66.0	&53.9	&61.8 \\
    Ours CoA/PGD-50 
    &74.5	&73.0	&75.8	&77.2	&68.0	&73.7 \\
    Ours CoA/PGD-100       
    &76.1	&74.4	&77.2	&78.5	&69.8	&75.2 \\

    \hline\hline 
        
\end{tabular}  
\end{threeparttable}  
\caption{pgd step}
\label{pgd step} 
\end{table*}

\begin{table*}[t]  

 %控制行高  
\setlength{\tabcolsep}{0.7mm}
\centering  
%\fontsize{9}{10}\selectfont  % \fontsize{字体尺寸}{行间距}\selectfont 
\begin{threeparttable}  
		  
%\begin{tabular}{cc|cccccc|ccc}  
%p{3cm} 
%>{\centering\arraybackslash}p{1.2cm} % 列居中+设定列宽为1.2cm
\begin{tabular}{c|cc|>{\centering\arraybackslash}p{1.4cm}>{\centering\arraybackslash}p{1.4cm}>{\centering\arraybackslash}p{1.4cm}>{\centering\arraybackslash}p{1.4cm}>{\centering\arraybackslash}p{1.4cm}>{\centering\arraybackslash}p{1.4cm}}  
    \toprule\hline
    \multirow{2}{*}{\bf \textsc{Vlm}}&
    \multirow{2}{*}{\bf \textsc{$\beta$}}&
    \multirow{2}{*}{\bf \textsc{$\gamma$}}&
    \multicolumn{6}{c}{\bf \textsc{CLIP Score / Text Encoder}}\cr

    %\cline{3-8}\cline{9-11}
    \cmidrule(lr){4-9}
    \multirow{6}{*}{\textsc{Unidiffuser} \cite{unidiffuser}} 
    &&&RN-50 & RN-101 & ViT-B/16 & ViT-B/32 & ViT-L/14 & Ensemble\\
    \hline
    &1 &1       
    &67.4	&65.2	&68.8	&70.6	&59.1	&66.2 \\
    &0.9 &0.1
    & 72.9	&71.7	&74.3	&75.4	&66.2	&72.1\\
    &0.8 &0.2 
    &73.3	&71.6	&74.5	&75.6	&66.3	&72.3 \\
    &0.7 &0.3
    &73.6	&71.9	&74.7	&75.8	&66.7	&72.5 \\
    &0.6 &0.4       
    &73.2	&71.5	&74.3	&75.4	&66.2	&72.1 \\

    \hline\hline 
        
\end{tabular}  
\end{threeparttable}  
\caption{TCM ablation}
\label{TCM ablaton} 
\end{table*}

\begin{table*}[t]  

 %控制行高  
\setlength{\tabcolsep}{0.7mm}
\centering  
%\fontsize{9}{10}\selectfont  % \fontsize{字体尺寸}{行间距}\selectfont 
\begin{threeparttable}  
		  
%\begin{tabular}{cc|cccccc|ccc}  
%p{3cm} 
%>{\centering\arraybackslash}p{1.2cm} % 列居中+设定列宽为1.2cm
\begin{tabular}{c|c|>{\centering\arraybackslash}p{1.4cm}>{\centering\arraybackslash}p{1.4cm}>{\centering\arraybackslash}p{1.4cm}>{\centering\arraybackslash}p{1.4cm}>{\centering\arraybackslash}p{1.4cm}>{\centering\arraybackslash}p{1.4cm}}  
    \toprule\hline
    \multirow{2}{*}{\bf \textsc{Vlm}}&
    \multirow{2}{*}{\bf \textsc{$\alpha$}}&
    \multicolumn{6}{c}{\bf \textsc{CLIP Score / Text Encoder}}\cr

    %\cline{3-8}\cline{9-11}
    \cmidrule(lr){3-8}
    \multirow{6}{*}{\textsc{ViECap} \cite{viecap}}  
    &&RN-50 & RN-101 & ViT-B/16 & ViT-B/32 & ViT-L/14 & Ensemble\\
    \hline
    &0.9        
    &77.6	&76.4	&78.6	&79.3	&71.6	&76.7 \\
    &0.7 
    &79.8	&80.4	&81.2	&81.5	&74.4	&79.0\\
    &0.5 
    &81.2	&80.4	&82.2	&83.0	&76.2	&80.6 \\
    &0.3 
    &82.7	&81.7	&83.6	&84.4	&78.1	&82.1 \\
    &0.1      
    &82.9	&81.9	&83.8	&84.7	&78.2	&82.3 \\

    \hline
    \multirow{6}{*}{\textsc{SmallCap} \cite{ramos2023smallcap}}
    &0.9        
    &68.4	&65.9	&69.4	&70.7	&59.9	&66.7 \\
    &0.7 
    &68.6	&66.1	&70.0	&71.1	&60.4	&67.2\\
    &0.5 
    &68.2	&65.7	&69.4	&70.7	&59.8	&66.8\\
    &0.3 
    &65.5	&62.6	&66.7	&68.1	&56.3	&63.8\\
    &0.1      
    &61.1	&58.2	&62.2	&63.7	&50.9	&59.2 \\
    
    \hline
    \multirow{6}{*}{\textsc{Unidiffuser} \cite{unidiffuser}} 
    &0.9        
    &73.6	&71.9	&74.7	&75.8	&66.7	&72.5 \\
    &0.7 
    &75.1	&73.3	&76.1	&77.2	&68.5	&74.0\\
    &0.5 
    &75.8	&74.3	&76.9	&78.1	&69.4	&74.9\\
    &0.3 
    &76.1	&74.4	&77.2	&78.5	&69.8	&75.2\\
    &0.1      
    &72.1	&70.5	&73.5	&75.1	&64.8	&71.2\\

    \hline\hline 
        
\end{tabular}  
\end{threeparttable}  
\caption{TCM ablation2}
\label{TCM ablaton2} 
\end{table*}
